# Supplementary material for: Leveraging Image Augmentation for Object Manipulation: Towards Interpretable Controllability in Object-Centric Learning
Source: arXiv:2310.08929 source file (2024-03-02)
Supplement: Supplementary file 1 [file eq_calibration.tex]

\begin{equation}
% \begin{split}
\vec{d} = (s - 1) (\vec{p} - \vec{c}),
% (d_x, d_y) = (s - 1) ((p_x, p_y) - (c_x, c_y))
% \end{split}
\label{eq:calibration}
\end{equation}
