# Supplementary material for: Leveraging Image Augmentation for Object Manipulation: Towards Interpretable Controllability in Object-Centric Learning
Source: arXiv:2310.08929 source file (2024-03-02)
Supplement: Supplementary file 2 [file eq_obj_level_loss_batch.tex]

\begin{equation}
% \begin{split}
\mathcal{L}_{\text{recon}} = \frac{1}{\mathcal{B}} \sum_{b=1}^{\mathcal{B}} \| \hat{\mathcal{I}}_{b} - \mathcal{I}_{b} \|_{2}^{2}
% \end{split}
\label{eq:line1}
\end{equation}

\begin{equation}
% \begin{split}
= \frac{1}{\mathcal{B}} \sum_{b=1}^{\mathcal{B}} \| \sum_{k=1}^{\mathcal{K}} (\hat{\mathcal{I}}_{b,k}^{rgb} \odot \hat{\mathcal{I}}_{b,k}^{\alpha}) - \mathcal{I}_{b} \|
% \end{split}
\label{eq:line2}
\end{equation}

\begin{equation}
% \begin{split}
= \frac{1}{\mathcal{B}} \sum_{b=1}^{\mathcal{B}} \| \sum_{k=1}^{\mathcal{K}} (\hat{\mathcal{I}}_{b,k}^{rgb} \odot \hat{\mathcal{I}}_{b,k}^{\alpha}) - \sum_{k=1}^{\mathcal{K}} (\mathcal{I}_{b} \odot \hat{\mathcal{I}}_{b,k}^{\alpha}) \|
% \end{split}
\label{eq:line3}
\end{equation}

\begin{equation}
% \begin{split}
= \frac{1}{\mathcal{B}} \sum_{b=1}^{\mathcal{B}} \sum_{k=1}^{\mathcal{K}} \| (\hat{\mathcal{I}}_{b,k}^{rgb} \odot \hat{\mathcal{I}}_{b,k}^{\alpha} - \mathcal{I}_{b} \odot \hat{\mathcal{I}}_{b,k}^{\alpha}) \|
% \end{split}
\label{eq:line4}
\end{equation}

% \begin{equation}
% % \begin{split}
% \approx \frac{1}{\mathcal{B}} \sum_{b=1}^{\mathcal{B}} \sum_{n=1}^{\mathcal{N}} \| (\hat{\mathcal{I}}_{b,n}^{rgb} \odot \hat{\mathcal{I}}_{b,n}^{\alpha} - \mathcal{I}_{b} \odot \hat{\mathcal{I}}_{b,n}^{\alpha}) \|
% % \end{split}
% \label{eq:line5}
% \end{equation}

\begin{equation}
% \begin{split}
\approx \frac{1}{\mathcal{B}} \sum_{b=1}^{\mathcal{B}} \sum_{k=1}^{\mathcal{K}}  \| \hat{\mathcal{O}}_{b,k} - \mathcal{O}_{b,k} \|
% \end{split}
\label{eq:lineX}
\end{equation}
