# Supplementary material for: Leveraging Image Augmentation for Object Manipulation: Towards Interpretable Controllability in Object-Centric Learning
Source: arXiv:2310.08929 source file (2024-03-02)
Supplement: Supplementary file 3 [file fig_cic.tex]

\begin{figure}
    \centering
    \includegraphics[width=\linewidth]{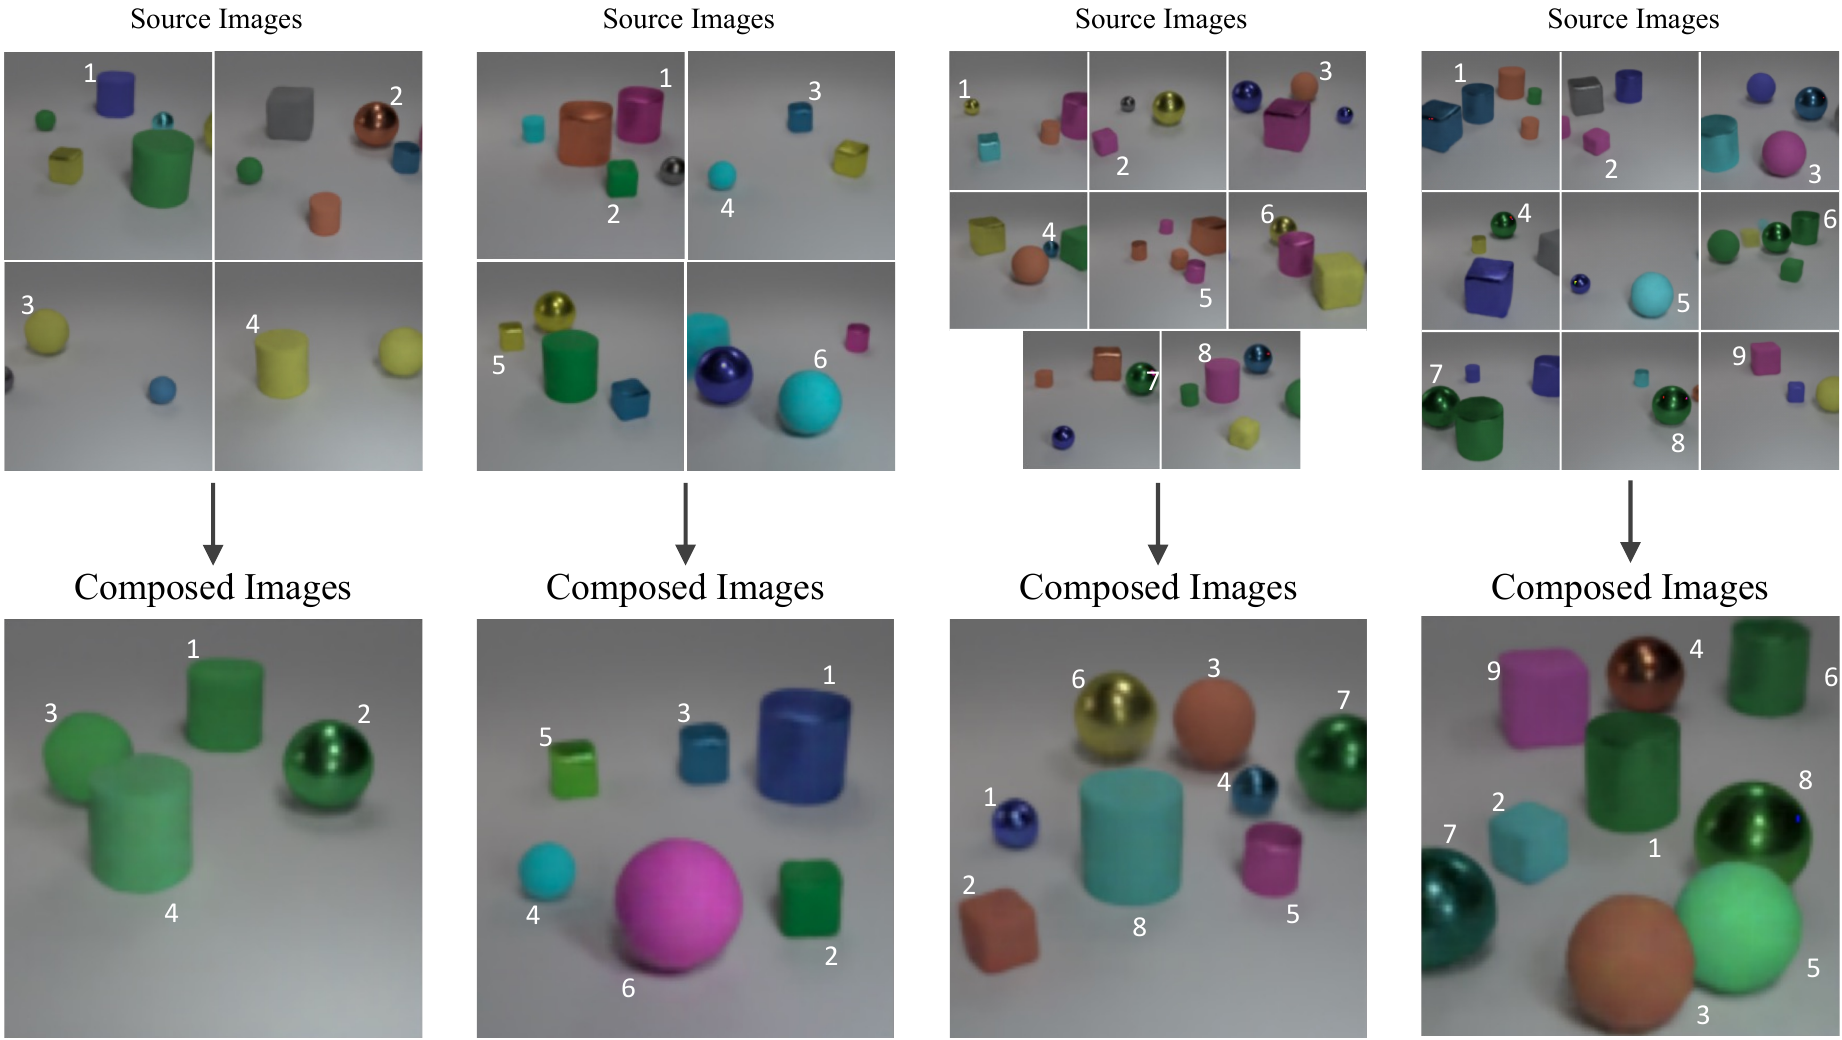}
    \vspace{-1em}
    \caption{ 
    Visualization of conditional image composition.
    The top row consists of the source images, while the bottom row displays the results of conditional image composition.
    }
    \label{fig:cic}
\end{figure}
