# Supplementary material for: Leveraging Image Augmentation for Object Manipulation: Towards Interpretable Controllability in Object-Centric Learning
Source: arXiv:2310.08929 source file (2024-03-02)
Supplement: Supplementary file 4 [file fig_unidec.tex]

\begin{figure}
    \centering
    \includegraphics[width=\linewidth]{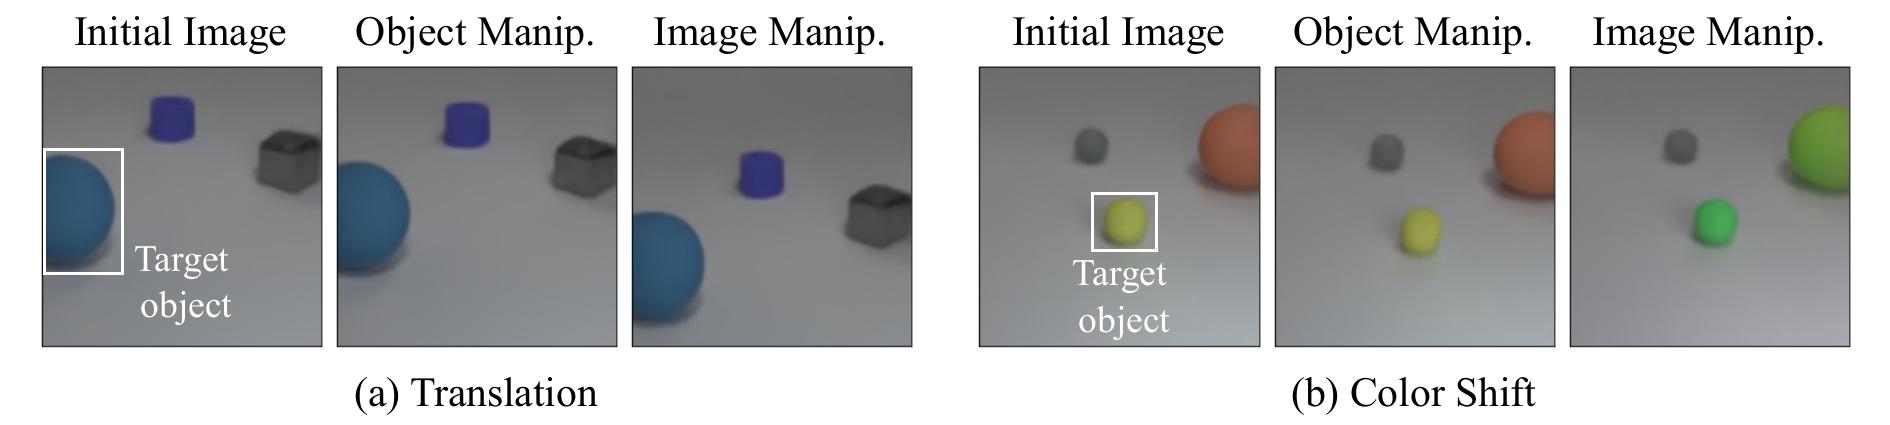}
    \vspace{-1em}
    \caption{ 
    Visualizations of object-level and image-level manipulations executed by SA-UniDec following two instructions: (a) translation, and (b) color shift. 
    For each instruction, the initial image, where the manipulation process begins, is positioned first, the image following object-level manipulation of the target object is placed second, and the image post image-level manipulation is situated third.
     To carry out image-level manipulation, we simply apply the same instructions uniformly to all slots, mirroring the manipulation process utilized during training.
    }
    \label{fig:unidec}
\end{figure}
