# Supplementary material for: Leveraging Image Augmentation for Object Manipulation: Towards Interpretable Controllability in Object-Centric Learning
Source: arXiv:2310.08929 source file (2024-03-02)
Supplement: Supplementary file 5 [file applications.tex]

\section{Application: object-centric image retrieval}

With the acquisition of controllability over object-centric representation, we can extend object-centric learning to two novel downstream tasks. 
\textit{Object-centric image retrieval} aims to retrieve an image having an object that is most relevant to a target object. 
In this task, we utilize object-centric representations acquired from given images as queries and keys to compute the object-level relevance score. 
The relevance score between a target and a candidate object can be computed by MSE or cosine similarity between the corresponding slots.

The retrieval process is as follows.
First, we acquire slots for a target object and candidate objects from the corresponding images by conducting object discovery.
Then, to reduce the effect of spatial properties such as object position and size, we \textit{neutralize} the slots by performing slot manipulation with the instructions for moving the objects to the central position and for scaling the objects to the unified size.
The 
After neutralization, the relevance score between the target slot and candidate slots is computed along the given metric.
Finally, object-centric image retrieval can be accomplished by finding the image containing the best-matched slot.
