# Supplementary material for: Leveraging Image Augmentation for Object Manipulation: Towards Interpretable Controllability in Object-Centric Learning
Source: arXiv:2310.08929 source file (2024-03-02)
Supplement: Supplementary file 6 [file failures.tex]

\section{Failure cases}
